# Supplementary material for: Search for $B_c^+\to\pi^+\mu^+\mu^-$ decays and measurement of the branching fraction ratio ${\cal B}(B_c^+\to\psi(2S)\pi^+)/{\cal B}(B_c^+\to J/\psi \pi^+)$
Source: arXiv:2312.12228 source file (2024-05-22)
Supplement: Supplementary file 1 [file appendix.tex]

% ===============================================================================
% Purpose: appendix to the standard template: standard symbol alises from Ulrik
% Author: Tomasz Skwarnicki
% Created on: 2009-09-24
% ===============================================================================

%{\noindent\normalfont\bfseries\Large Appendices}
\section*{Appendices}

\appendix
